# Supplementary material for: Slow modulation of the contraction patterns in Physarum polycephalum
Source: arXiv:2501.02651 source file (2025-09-20)
Supplement: Supplementary file 1 [file Supplementary__Saiseau2025_Physarum_Modulation.pdf]

# Supplementary Materials – Slow modulation of the contraction patterns in *Physarum polycephalum*

Raphael Saiseau,[1,2,*] Valentin Busson,[1] and Marc Durand[1,†]

[1] *Laboratoire MSC, Université Paris Cité, CNRS, UMR 7057, Matière et Systèmes Complexes (MSC), F-75006 Paris, France.*

[2] *Department of Physics, University of Konstanz, 78457 Konstanz, Germany*

## I. MATERIALS AND METHODS

### A. Experimental system culture and insemination

Experiments were conducted on *Physarum polycephalum* in its plasmodial stage, obtained as sclerotia (Carolina Biological, USA). Plasmodia were grown on Petri dishes half filled with Phytagel-based gels, containing glucose kept at a sufficiently low concentration to avoid bias caused by chemotaxis. Gels are composed of 2% Phytagel, 1% glucose, and can include 2% oatmeal agar, to test nutrient availability effect [1]. No systematic differences were observed when adding oatmeal. Cultures were fed with sterilized oat flakes and kept at 25°C in darkness. Once or twice per week, the growing front was transferred to fresh gel. After 10–20 h of recovery and spreading, ring-shaped plasmodia were prepared by punching concentric annuli with thin plastic rings, which remained in place to prevent fusion. This procedure defined annuli with perimeters $L = 6.0$–$13.5$ cm and aspect ratios $L/e = 11$–$41$, where $e$ is annulus width. Dishes were sealed and maintained at 25°C with heating plates during recordings. Transmitted light microscopy video is started after a typical settling time of 15–30 minutes.

### B. Image acquisition

Ring plasmodia were imaged in transmitted light using a Leica Z16 APO macroscope with TL5000 LED base (440–650 nm) and a CMOS Basler acA2440-75uc color camera. Intensity has been dimmed at its maximum to ensure that it does not elicit a specific response from the plasmodium [2]. RGB images were recorded every 4–6 s with ∼500 ms exposure, 37 $\mu$m/pixel resolution (2448×2048 pixels), for total film durations of 4–15 h. All experiments were conducted in a light-tight enclosure.

### C. Beer-Lambert law

To relate transmitted intensity to cytoplasm thickness, we placed plasmodium samples in a custom-built glass wedge chamber of controlled gradient thickness. Intensity measurements were fitted with the Beer–Lambert law,

$$I = I_0 e^{-h/\ell_a}, \tag{1}$$

yielding absorption lengths $\ell_a \simeq 100$ $\mu$m (blue), 200 $\mu$m (green), and 350 $\mu$m (red), which vary slightly due to the aging of Physarum pigments. These values are consistent with measurements ($\ell_a \simeq 67$ $\mu$m) reported by Bykov et al. [3] obtained with a Doppler optical coherence tomography technique with an infrared (840 $nm$) superluminescent diode. The blue channel, providing highest sensitivity, was used in subsequent analysis.

### D. Signal analysis

Height variations were obtained from transmitted intensity using the Beer–Lambert calibration (blue channel). The signal was smoothed with a 10-frame (∼60 s) top-hat filter to remove high-frequency noise. At each position, the height was decomposed as

$$h(t) = D(t) + A(t)\cos\phi(t), \tag{2}$$

where $D(t)$ is the slow baseline drift (vein diameter and network reorganisation), $A(t)$ the oscillation amplitude (modulated on intermediate timescales), and $\phi(t)$ the instantaneous phase (fast contractile state). Signal upper and lower envelopes were extracted by cubic spline interpolation of extrema, defining $h_{\max}(t)$ and $h_{\min}(t)$, respectively. The drift $D(t)$ and amplitude $A(t)$ are then defined as:

$$D(t) = (h_{\max}(t) + h_{\min}(t))/2, \tag{3}$$

$$A(t) = (h_{\max}(t) - h_{\min}(t))/2. \tag{4}$$

The phase $\phi(t)$ was computed as the argument of the analytic signal obtained from the Hilbert transform of $(h - D)/A$ [4]. Values were averaged over an angular sector. Angular sectors are of constant arc length ($\simeq 1.1$ mm) by adjusting the number of sectors $N$ according to the ring perimeter $L$.

### E. Pattern classification.

Spatio-temporal patterns (rotating vs alternating/standing) were identified by visual inspection of

* raphael.saiseau@uni-konstanz.de

† marc.durand@univ-paris-diderot.fr

amplitude kymographs. Patterns classified as *rotating* show clear slanted isophase contours traveling around the ring, while *alternating/standing* patterns exhibit persistent nodes and horizontally aligned envelopes. Representative kymographs illustrating rotating and alternating modes are provided in the main text (Figs. 2(c-e), 3(a), and 4(a)), and the raw time-series and kymograph-generation code are available in the project repository to allow independent verification.

## II. SUPPLEMENTARY FIGURES

### Figure S1: Change of rotation for signal modulation Patterns

Here we show an example of a sudden change of rotation direction in a rotating modulation pattern.

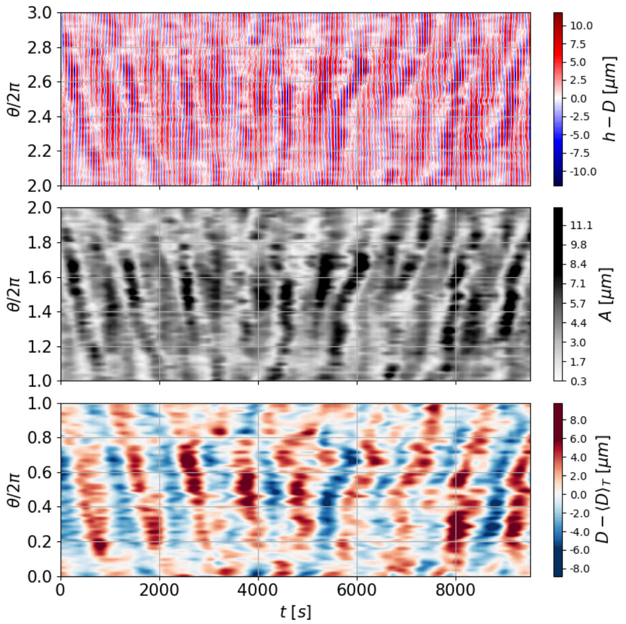


Height variations, amplitude and drift mapping over angle and time, showing a rotating pattern that abruptly changes rotation direction.

**Figure S2: Modulation signals for cut organisms**

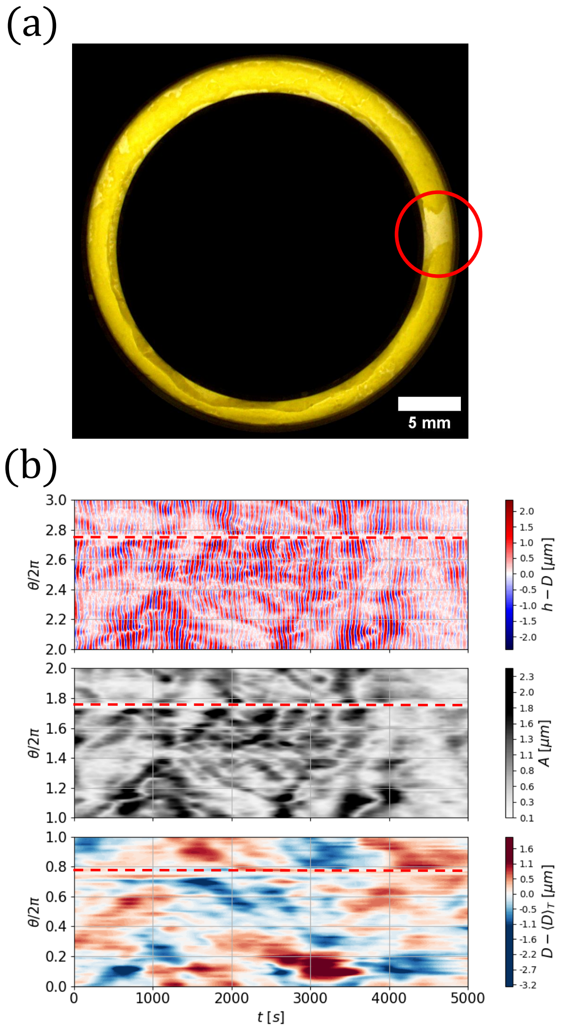


(a) Bright-field image of a ring with a cut section (red dashed circle). (b) Time series of $h$, $A$, and $D$ for this ring: long-range spatio-temporal coordination is absent in the presence of architectural damage.

**Figure S3: Modulation signals for organisms with dying/drying section**

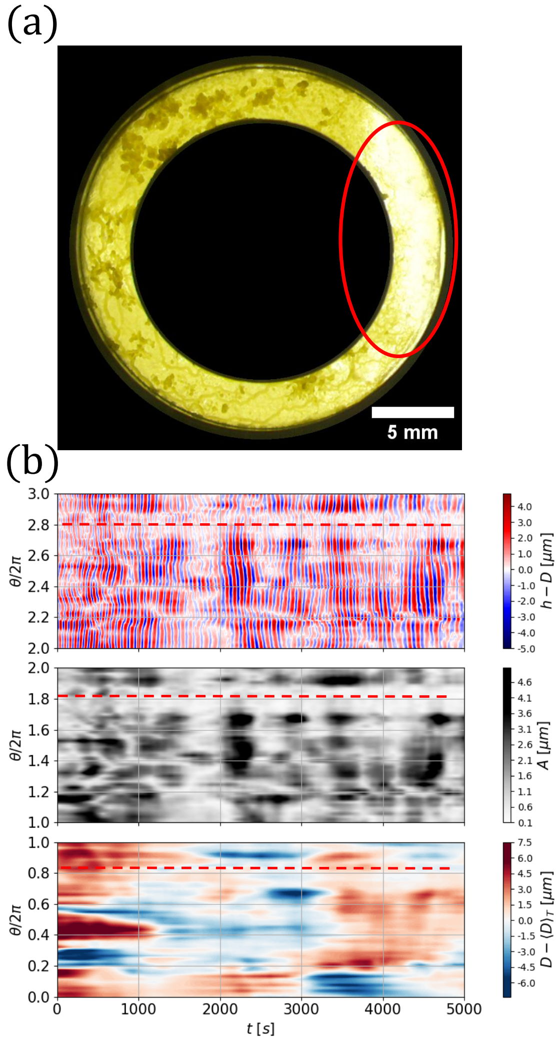


(a) Bright-field image of a ring with a dying/drying section. (b) Corresponding $h$, $A$, and $D$: loss of long-range modulation is observed when a region dries or dies.

**Figure S4: Additional network examples**

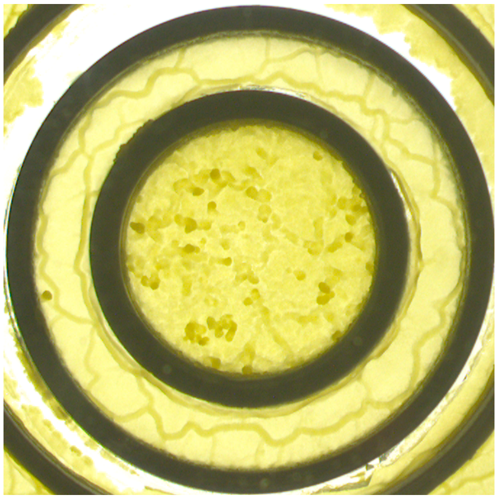

(a)

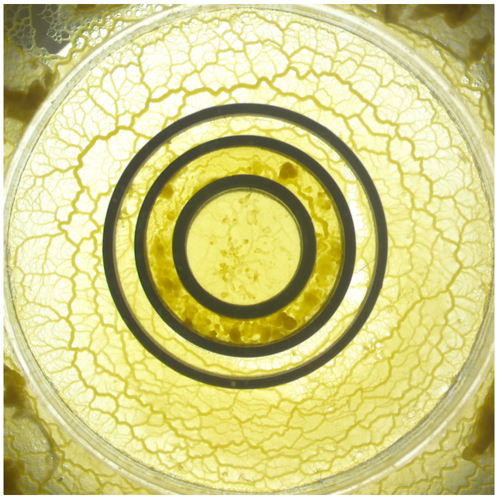

(b)

Examples of ring-confined networks corresponding to (a) a rotating pattern and (b) an alternating/internal pattern. Networks showing well-developed central veins tend to present the large-scale rotating modes.

[1] A. Dussutour, T. Latty, M. Beekman, and S. J. Simpson, Amoeboid organism solves complex nutritional challenges, Proceedings of the national academy of sciences **107**, 4607 (2010).

[2] M. Hato, T. Ueda, K. Kurihara, and Y. Kobatake, Phototaxis in true slime mold physarum polycephalum, Cell Structure and function **1**, 269 (1976).

[3] A. V. Bykov, A. V. Priezzhev, J. Lauri, and R. Myllylä, Doppler oct imaging of cytoplasm shuttle flow in physarum polycephalum (2009).

[4] P. Etévenon, N. Lebrun, P. Clochon, G. Perchey, F. Eustache, and J.-C. Baron, High temporal resolution dynamic mapping of instantaneous eeg amplitude modulation after tone-burst auditory stimulation, Brain Topography **12**, 129 (1999).
